# Supplementary material for: Generative Quanta Color Imaging
Source: arXiv:2403.19066 source file (2024-03-28)
Supplement: Supplementary file 1 [file X_suppl.tex]

\clearpage
\setcounter{page}{1}
\appendix
\maketitlesupplementary
\setcounter{table}{0}
\setcounter{equation}{0}
\setcounter{figure}{0}
\section*{A1 - Proof of Theorem 3.1}\label{sec:theorem_proof}
 Given a 1bQIS image $\mathbf{Y}(u)$ where $u \in \mathcal{U}$ and $\mathcal{U} \subset \mathbb{Z}^2$, we have the local bit density $\mu\propto\|x\|_2$, where $\|\mathbf{Y}\|_{2}^{2} := \sum_{u^{'} \in N_u}\mathbf{Y}(u - u^{'})^{2}$, and $N_u$ is a local Euclidean grid centered at $u$. Then the output of $\ell$-th layer of CNN layer can  be written as,
        \begin{equation}
            \textbf{Y}^{\ell}(u) =  \sigma(\sum_{k=1}^{m} \mathbf{\phi}_{k}^{\ell} \langle \textbf{x}^{\ell-1}, \mathbf{\Lambda}^{\ell,k} \rangle_{N_u} + b^{\ell}),
            \vspace{-1mm}
        \end{equation}
        where $\sigma$ is nonlinear mapping such as ReLU which is non-expansive, $\mathbf{\Lambda}^{\ell,k}$ represents $k$-{th} atoms in $\ell$-th layer, $\mathbf{\phi}_{k}^{\ell}$ corresponds to $k$-th coefficient, and $b^{\ell}$ is the bias of $\ell^{th}$ layer.
\begin{theorem} 
    If $\mathbf{\Lambda}_1$ and $\mathbf{\Lambda}_2$ are filter atoms generated with neural ODE using integration intervals ($\widetilde{\theta}_{\text{0}}$, $\widetilde{\theta}_{\text{1}}$) and ($\widetilde{\theta}_0,\widetilde{\theta}_2$), respectively such that $\|\mathbf{\Lambda}_1 - \mathbf{\Lambda}_2  \| \leq \epsilon|\widetilde{\theta}_1 - \widetilde{\theta}_2|$, for $\epsilon > 0$. If $\theta_1$ and $\theta_2$ are the exposures at $\widetilde{\theta}_1$ and $\widetilde{\theta}_2$, and activation function $\sigma$ is non-expansive, then change in quanta exposure $\Delta \theta$ is continuous in filter atoms.
    \label{thm}
\end{theorem} 
\textbf{Proof.} As the result of atom-coefficient decomposition, a convolutional kernel of $\ell^{th}$ layer is $f_{\ell} = \mathbf{\phi}^{\ell}\mathbf{\Lambda}^{\ell}(\widetilde\theta)$, where $\mathbf{\Lambda}^{\ell}(\widetilde\theta)$ corresponds to the atoms responsible for generating image with exposure $\widetilde\theta$ and $\mathbf{\phi}^{\ell}$ corresponds to coefficients. The result of convolution operation on feature map $\mathbf{Y}^{\ell-1}$ from previous layer is given by -
\begin{equation}
    \mathbf{Y}^{\ell} = f_{\ell}(\mathbf{Y}^{\ell-1}, \mathbf{\Lambda}^{\ell}(\widetilde\theta), \mathbf{\phi}^i) =  \sigma(\sum_{k=1}^{m} \mathbf{\phi}_{k}^{\ell} \langle \textbf{x}^{\ell-1}, \mathbf{\Lambda}^{\ell,k} \rangle_{N_u} + b^{\ell}).
\end{equation}
With sigma being non-expansive we can write (ignoring bias $b_{\ell}$ for simplicity ) -
\begin{equation}
    |\mathbf{Y}^{\ell}_{1}(u) -  \mathbf{Y}^{\ell}_{2}(u)| \leq |  \sum_{i=1}^k \mathbf{\phi}^{\ell}_{i} \langle  {\mathbf{Y}^{\ell-1}},\mathbf{\Lambda}^{\ell}_{1}(\widetilde\theta_{1}) \rangle_{N_u} - \sum_{i=1}^k \mathbf{\phi}^{\ell}_{i} \langle  {\mathbf{Y}^{\ell-1}},\mathbf{\Lambda}^{\ell}_{2}(\widetilde\theta_{2}) \rangle_{N_u}| \leq \sum_{i=1}^k | \mathbf{\phi}^{\ell}_{i} [ \langle {\mathbf{Y}^{\ell-1}},\mathbf{\Lambda}^{\ell-1}_{1}(\widetilde\theta_{1}) \rangle_{N_u} - \langle {\mathbf{Y}^{\ell-1}},\mathbf{\Lambda}^{\ell}_{2}(\widetilde\theta_{2}) \rangle_{N_u}]|,
\end{equation}
let $B^{\ell} = [\langle {\mathbf{Y}^{\ell-1}},\mathbf{\Lambda}^{\ell}_{1}(\widetilde\theta_{1}) \rangle_{N_u} - \langle {\mathbf{Y}^{\ell-1}},\mathbf{\Lambda}^{\ell}_{2}(\widetilde\theta_{2}) \rangle_{N_u}]$. Then we have, 
\begin{equation}
    |\mathbf{Y}^{\ell}_{1}(u) -  \mathbf{Y}^{\ell}_{2}(u)| \leq \sum_{i=1}^k | \mathbf{C}^{\ell}_{i} B^{\ell}_{i}|,
\end{equation}
Using H\"{o}lder's inequality with $p=2$ and $q=2$ -
\begin{equation}
\begin{split}
    |\mathbf{Y}^{\ell}_{1}(u) -  \mathbf{Y}^{\ell}_{2}(u)|  & \leq (\sum_{i=1}^k(|\mathbf{\phi}^{l}_i|^2)^{\frac{1}{2}}) \sum_{k=1}^k(|B^{l}_i|^2)^{\frac{1}{2}},\\
    & \leq \|\mathbf{\phi}^{\ell}\|_2 \sum_{i=1}^k(|B^{l}_i|^2)^{\frac{1}{2}}.
\end{split}
\end{equation}
Consider only 2nd term in above equation $\sum_{i=1}^k(|B^{l}_i|^2)^{\frac{1}{2}} = \sum_{i=1}^k(| \langle {\mathbf{Y}^{\ell-1}},\mathbf{\Lambda}^{\ell}_{1}(\widetilde\theta_{1}) \rangle_{N_u} - \langle {\mathbf{Y}^{\ell-1}},\mathbf{\Lambda}^{\ell}_{2}(\widetilde\theta_{2}) \rangle_{N_u}|^2)^{\frac{1}{2}}$. Then,
\begin{equation}
    | \langle {\mathbf{Y}^{\ell-1}},\mathbf{\Lambda}^{\ell}_{1}(\widetilde\theta_{1}) \rangle_{N_u} - \langle {\mathbf{Y}^{\ell-1}},\mathbf{\Lambda}^{\ell}_{2}(\widetilde\theta_{2}) \rangle_{N_u}|^2 \leq | \langle {\mathbf{Y}^{\ell-1}},(\mathbf{\Lambda}^{\ell}_{1}(\widetilde\theta_{1})  -\mathbf{\Lambda}^{\ell}_{2}(\widetilde\theta_{2})) \rangle_{N_u}|^2.
\end{equation}
Using Cauchy-Schwarz inequality -
\begin{equation}
    | \langle {\mathbf{Y}^{\ell-1}},(\mathbf{\Lambda}^{\ell}_{1}(\widetilde\theta_{1})  -\mathbf{\Lambda}^{\ell}_{2}(\widetilde\theta_{2})) \rangle_{N_u}| \leq \|\mathbf{Y}^{\ell-1}\|_{2, N_u} . \|\mathbf{\Lambda}^{\ell}_{1}(\widetilde\theta_{1})  -\mathbf{\Lambda}^{\ell}_{2}(\widetilde\theta_{2})\|_{2}.
\end{equation}
Substituting results from Eq. 5 and 6 into Eq. 4 -
\begin{equation}
\begin{split}
    |\mathbf{Y}^{\ell}_{1}(u) -  \mathbf{Y}^{\ell}_{2}(u)| & \leq  \|\mathbf{\phi}^{\ell}\|_2 . \sum_{i=1}^k \bigg(\|\mathbf{Y}^{\ell-1}\|_{2, N_u}^2 . ||\mathbf{\Lambda}^{\ell}_{1}(\widetilde\theta_{1})  -\mathbf{\Lambda}^{\ell}_{2}(\widetilde\theta_{2})\|_{2}^2\bigg)^{\frac{1}{2}}, \\ 
    & \leq  \|\mathbf{\phi}^{\ell}\|_2 \|\mathbf{Y}^{\ell-1}\|_{2, N_u} \sum_{i=1}^k \|\mathbf{\Lambda}^{\ell}_{1}(\widetilde\theta_{1})  -\mathbf{\Lambda}^{\ell}_{2}(\widetilde\theta_{2})\|_{2}.
\end{split}
\end{equation}

\begin{equation}
    \sum_{u \in \mathcal{S}} |\mathbf{Y}^{\ell}_{1}(u) -  \mathbf{Y}^{\ell}_{2}(u)|^2 \leq   \|\mathbf{\phi}^{\ell}\|_2^2 \|\mathbf{Y}^{\ell-1}\|_{2, N_u}^2 \sum_{u}  \sum_{i=1}^k \|\mathbf{\Lambda}^{\ell}_{1}(\widetilde\theta_{1})  -\mathbf{\Lambda}^{\ell}_{2}(\widetilde\theta_{2})\|_{2}.
\end{equation}
Note that - 
\begin{equation}
    \sum_{u}  \sum_{i=1}^k \|\mathbf{\Lambda}^{\ell}_{1}(\widetilde\theta_{1})  -\mathbf{\Lambda}^{\ell}_{2}(\widetilde\theta_{2})\|_2 = \sqrt{ |\mathcal{U}|} .  \|\mathbf{\Lambda}^{\ell}_{1}(\widetilde\theta_{1})  -\mathbf{\Lambda}^{\ell}_{2}(\widetilde\theta_{2})\|_{2},
\end{equation}
with $|\mathcal{U}|$ being the domain of $\mathbf{Y}^{\ell-1}$. Then Eq.8 becomes - 
\begin{equation}
    \|\mathbf{Y}^{\ell}_{1} -  \mathbf{Y}^{\ell}_{2}\|_{2} \leq \|\mathbf{\phi}^{\ell}\|_2 \|\mathbf{Y}^{\ell-1}\|_{2, N_u} \sqrt{|\mathcal{U}|} \cdot \|\mathbf{\Lambda}^{\ell}_{1}(\widetilde\theta_{1})  -\mathbf{\Lambda}^{\ell}_{2}(\widetilde\theta_{2})\|_{2}.
\end{equation}
Since the bit density of 1bQIS is the average number of ones in the space-time volume. Hence $\|\mathbf{Y}\|_2 \propto \mu$.  Then, 
\begin{equation}
     \|\mu_{1}^{l} - \mu_{2}^{l} \|_2 \leq \|\mathbf{\phi}^{\ell}\|_2 \|\mathbf{Y}^{\ell-1}\|_{2, N_u} \sqrt{|\mathcal{U}|} \cdot \|\mathbf{\Lambda}^{\ell}_{1}(\widetilde\theta_{1})  -\mathbf{\Lambda}^{\ell}_{2}(\widetilde\theta_{2})\|_{2}.
\end{equation}
Since bit density is the sufficient statistic of exposure $\boldsymbol{\theta}$, We can write - 
\begin{equation}
    \|\boldsymbol{\theta}_{1}^{l} - \boldsymbol{\theta}_{2}^{l}\|_2 \leq \|\mathbf{\phi}^{\ell}\|_2 \|\mathbf{Y}^{\ell-1}\|_{2, N_u} \sqrt{|\mathcal{U}|} \cdot \|\mathbf{\Lambda}^{\ell}_{1}(\widetilde\theta_{1})  -\mathbf{\Lambda}^{i}_{2}(\widetilde\theta_{2})\|_{2}.
\end{equation}
\section*{A2 - Architecture, Hyper-parameters, Synthetic Data Generation and Benchmarks}
\subsection*{A2.0 - Details About Comparison With Image Augmentation Approach}
For the results presented in \cref{fig:colorize pipelines}, we compare the performance of image augmentation without exposure correction against our method. During the training phase of the colorizer, we augment the dataset with images from an exposure spectrum of $\tau = \{5, 10, 15\}$. However, for the exposure correction-based approach, we use the same exposure levels but do not perform dataset augmentation. Both methods are trained for similar number of iterations and tested on images with an exposure of $\tau = 0$ to ensure fair comparison. 
\subsection*{A2.1 - Architecture}
In this section, we detail the architectures used for exposure correction, Single Image Colorization (SIC) and Burst Image Colorization (BIC).
\subsubsection*{A2.1.1 - AtomODEPix2Pix and AtomODECycle}
The AtomODE-Pix2Pix and AtomODE-Cycle are modified versions of Pix2Pix \cite{isola2017image} and CycleGAN \cite{zhu17} respectively. The key difference between Pix2Pix and AtomODE-Pix2Pix lies in the bottleneck layer of the generator. We substitute the convolutional layers in the generator with Exposure Adaptive Convolutional Layer (EACL). For NeuralODE we design 6 layers of [GroupNorm, Activation, Convolutional Layer]. We use Tanh as activation function. We use $\text{rtol}=1 \mathrm{x}10^{-3}$ and $\text{atol}=1 \mathrm{x}10^{-3}$. We use a multiscale discriminator for both AtomODEPix2Pix and AtomODECycle. Further, we provide a detailed account of the hyperparameters in Section S3.2.
\subsubsection*{A2.1.2 - Pix2PixFuse}
Pix2PixFuse inherits the meta-architecture from Pix2Pix with an additional Cross Non-Local Fusion (CNLF) \cite{Luo_2021_CVPR} block. We use CNLF block to constructively fuse the representations obtained from images of different exposures. In Figure \ref{fig:pix2pixfuse_arch} shows the Pix2PixFuse architecture.
\begin{figure}
          \centering
           \includegraphics[scale=0.2]{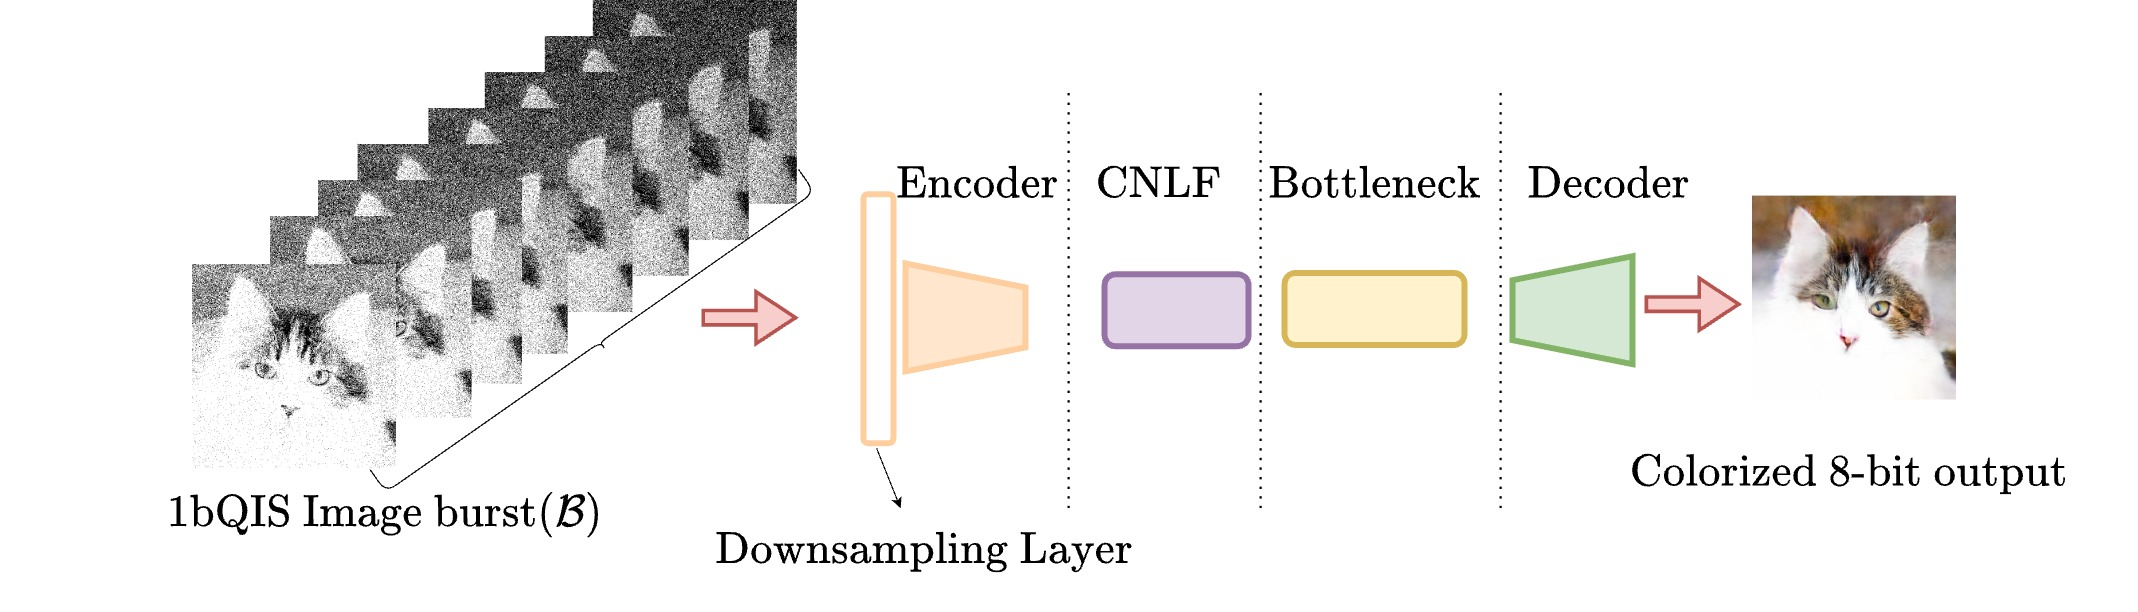}
           \caption{Pix2PixFuse for burst image colorization.}
           \label{fig:pix2pixfuse_arch}
\end{figure}
\subsection*{A2.2 - Hyper-parameters}\label{sec:hypers}
\begin{table}[]
\resizebox{\textwidth}{!}{
\begin{tabular}{lll}
\hline
\multicolumn{1}{c}{\multirow{2}{*}{Hyperparameters}}            & \multicolumn{2}{c}{\textbf{Exposure Correction Methods}}                                           \\ \cline{2-3} 
\multicolumn{1}{c}{}                                            & \textbf{AtomODE Pix2Pix}    & \textbf{AtomODE-CycleGAN} \\ \hline
Input image dimension (\# of images, \#channels, height, width) & 1, 1, 512, 512 or 1,1,256, 256               & 1, 1, 512, 512 or 1,1,256,256              \\
learning rate                                                   & 0.00002                                      & 0.00002                                    \\
norm                                                            & BatchNorm and GroupNorm(Neural ODE) & batch and GroupNorm(Neural ODE)   \\
dropout rate                                                    & 0.5                                          & 0.5                                        \\
batchsize                                                       & 1                                            & 1                                          \\
input number of channels                                        & 1                                            & 1                                          \\
output number of channels                                       & 1                                            & 1                                          \\
serial batches                                                  & True                                         & False                                      \\
no-flip                                                         & True                                         & True                                       \\
netG                                                            & ResNet-9                                     & ResNet-9                                   \\
\# of filter in first layer of generator                        & 64                                           & 64                                         \\
\# of blocks in generator                                       & 9                                            & 9                                          \\
number of epochs                                                & 100                                          & 100                                        \\
optimizer                                                       & Adam                                         & Adam                                       \\
betas                                                           & (0.5, 0.999)                                 & (0.5, 0.999)                               \\
Discriminator type                                              & Multiscale                                   & Multiscale                                 \\
\# of discriminators                                            & 2                                            & 2                                          \\
\# of layers in discriminators                                  & 3                                            & 3                                          \\
\# of filter in first layer of discriminator                    & 64                                           & 64                                         \\
weight for feature matching loss                                & 0                                            & 0                                          \\
Adverserial loss                                                & True                                         & True                                       \\
VGG loss                                                        & False                                        & False                                      \\
GAN type                                                        & Vanilla GAN                                  & Vanilla GAN                                \\
activation                                                      & sigmoid and Tanh (only for Neural ODE)       & sigmoid and Tanh (only for Neural ODE)     \\ \hline
\end{tabular}
}
\caption{Hyperparameter table for AtomODE Pix2Pix, AtomODE CycleGAN.}
\label{tab:exposure_para}
\end{table}

\begin{table}[]
\resizebox{\textwidth}{!}{%
\begin{tabular}{lll}
\hline
\multicolumn{1}{c}{Hyperparameters}                             & \textbf{Single Image Colorizer} & \textbf{Burst Image Colorzier}                 \\ \cline{2-3} 
                                                                & \textbf{Pix2Pix}                & \textbf{Pix2PixFuse} \\ \hline
Input image dimension (\# of images, \#channels, height, width) & 1, 1, 512, 512 or 1,1,256,256                    & N, 1, 512, 512                        \\
learning rate                                                   & 0.0002                                           & 0.0002                                \\
norm                                                            & BatchNorm                                        & BatchNorm                             \\
dropout rate                                                    & 0.5                                              & 0.5                                   \\
batchsize                                                       & 6                                                & 1                                     \\
input number of channels                                        & 1                                                & 1                                     \\
output number of channels                                       & 3                                                & 3                                     \\
serial batches                                                  & True                                             & True                                  \\
no-flip                                                         & True                                             & True                                  \\
netG                                                            & ResNet-9                                         & ResNet-9 + CNLF                       \\
\# of filter in first layer of generator                        & 64                                               & 64                                    \\
\# of blocks in generator                                       & 9                                                & 9                                     \\
number of epochs                                                & 250                                              & 100                                   \\
optimizer                                                       & Adam                                             & Adam                                  \\
betas                                                           & (0.5, 0.999)                                     & (0.5, 0.999)                          \\
Discriminator type                                              & Multiscale                                       & Multiscale                            \\
\# of discriminators                                            & 2                                                & 2                                     \\
\# of layers in discriminators                                  & 3                                                & 3                                     \\
\# of filter in first layer of discriminator                    & 64                                               & 64                                    \\
weight for feature matching loss                                & 0                                                & 0                                     \\
Adverserial loss                                                & True                                             & True                                  \\
VGG loss                                                        & True                                             & True                                  \\
GAN type                                                        & Vanilla GAN                                      & Vanilla GAN                           \\
activation                                                      & sigmoid                                          & sigmoid                               \\ \hline
\end{tabular}
}
\caption{Hyperparameter table for SIC and BIC architectures.}
\label{tab:colorizer_hyper}
\end{table}
The hyperparameters used by different architectures are shown in Table \ref{tab:exposure_para} and Table \ref{tab:colorizer_hyper}. AtomODE-Pix2Pix and AtomODE-CycleGAN are trained on 24GB Nvidia 3090Ti GPU and rest of the models are trained on V100.
\subsection*{A2.3 - Additional Details About Benchmarks}
In this section, we provide additional training details about the benchmarks we used to compare our algorithm. 
\begin{itemize}
    \item \textbf{DLOW}: DLOW is a continuous model by design. We train it with $\tau = 0$ exposure image as the input domain and $\tau = 14$ as the target domain.  We supply images from the intermediate domains $\tau = {4, 9}$ for additional guidance. The model was trained for 100 epochs with a learning rate of  0.0002, batch size 1.  DLOW uses cycleGAN architecture and is trained using unpaired data setting. 
    \item \textbf{Pix2PixDNI}: Deep Network Interpolation to interpolate among kernels of finetuned networks for continuous i2i. We train two models that translate input image $\tau = 0$ to $\tau = 9$ and from $\tau = 0$ to $\tau=14$. We interpolate between these two models to obtain multiple models that translate input ($\tau = 0$) to $\tau = \{k\}_{k=1}^14$. We use Pix2Pix architecture using paired data setting. All the other hyper-paramters remain similar to AtomODE-Pix2Pix. 
    \item \textbf{CycleDNI}: Deep Network Interpolation to interpolate among kernels of finetuned networks for continuous i2i. We train two models that translate input image $\tau = 0$ to $\tau = 9$ and from $\tau = 0$ to $\tau=14$. We interpolate between these two models to obtain multiple models that translate input ($\tau = 0$) to $\tau = \{k\}_{k=1}^14$. We use CycleGAN architecture using unpaired data setting. All the other hyper-paramters remain similar to AtomODE-CycleGAN.
    \item \textbf{SAVI2I} : SAVI2I synthesizes intermediate results between two domains. In our case, the input domain image belongs to $\tau = 0$ and output domain $\tau = 14$. We do not use style reconstruction loss as it led to inferior results.
\end{itemize}

\subsection*{A2.4 - Synthetic Data Generation}
In this section, we detail the generation of 1bQIS versions of AFHQ and CelebA datasets from their RGB counterpart. In Figure \ref{fig:imaging_model}, we show a simplified imaging model of 1bQIS. Following are the steps followed for generating burst of 1bQIS images with varying exposures from a single RGB image. 

\begin{itemize}
\item\textbf{Step 1 :} Extract quanta exposure $\boldsymbol{\theta}$ from RGB images.

\item\textbf{Step 2 :} We simulate exposure bracketing to generate burst of 1bQIS images with varying burst. To this end, we divide the overall exposure ($\boldsymbol{\theta}$) into brackets. The bracketing is controlled using the parameter $\alpha$. $\alpha$ varies between (1, 25) with a difference of 0.5, set of all such $\alpha = \{1.0, 1.5, 2.0, 2.5, 3.0, 3.5, 4.0, 4.5, 5.0, 5.5, 6.0, 6.5, 7.0,7.5, 8.0 \}$.Let the exposure obtained by dividing $\alpha_i$ be $\boldsymbol{\theta}_{i}$. In summary we obtain a set of exposures $\{\boldsymbol{\theta_i}\}_{i=0}^{14}$ using set of  $\{\alpha_i\}_{i=0}^{14}$.

\item\textbf{Step 3 :} 
Using the set of $\alpha$ in Step 2, obtain the binary measurements following the imaging model of 1bQIS. If $\mathbf{X} = \mathrm{Poisson}(\boldsymbol{\theta}_i) + \mathrm{Gaussian}(0, \sigma^2)$ be the measurements before binarization and let $\mathbf{Y}$ denote the binarized output. $Y$ is assigned a value of ``1" if $\mathbf{X} \geq q$ else ``0". We use $q = 0.5$ to generate the synthetic data.

\item\textbf{Step 4 :} In the synthetic dataset, we have an exposure burst going from overexposed $\rightarrow$ underexposed for each image. There is a total of 15 images in each burst and we show one such burst in Figure \ref{fig:eg_burst}. All the images in a burst are indexed using an indexing variable $\tau$. We assign a continuous variable $\widetilde\theta \in (0,1)$. For example, the assigned continuous variable $\widetilde\theta$ for the example exposure spectrum is shown in Figure \ref{fig:eg_burst} is - $\{0.0625, 0.125, 0.1875, 0.25, 0.3125, 0.375, 0.4375, 0.5, 0.5625, 0.625, 0.6875, 0.75, 0.8125, 0.875, 0.9375\}$
\end{itemize}
\begin{figure}
  \centering
\includegraphics[width=0.6\textwidth,height=0.6\textheight,keepaspectratio]{sec/figs/imaging_model.jpg}
   \caption{1bQIS imaging model showing multiple output binary images of the same scence.}
   \label{fig:imaging_model}
\end{figure}
\begin{figure}
  \centering
\includegraphics[width=0.8\textwidth,height=0.8\textheight,keepaspectratio]{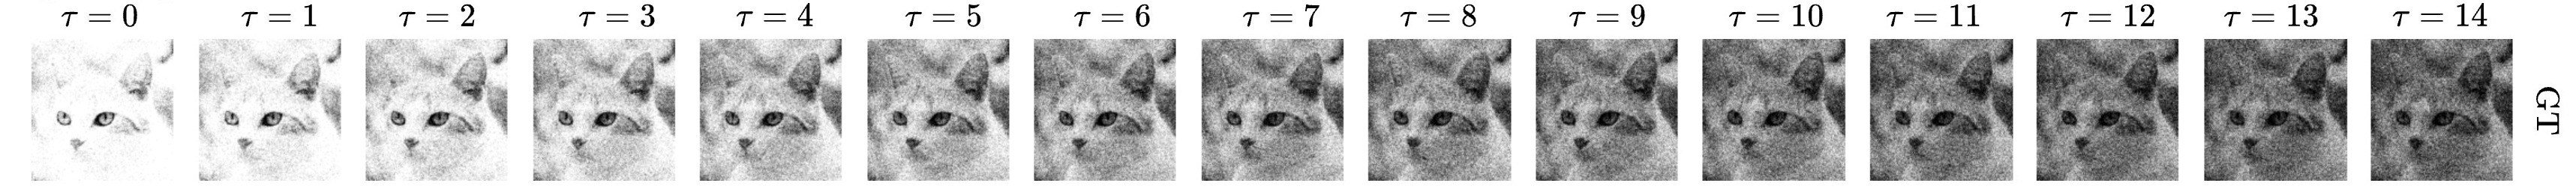}
   \caption{An example exposure burst.}
   \label{fig:eg_burst}
\end{figure}
\section*{A3 - Assumptions and Drawbacks}
We make following assumptions for our method to work -
\begin{itemize}
    \item In the main paper, we showed the burst recovery using an overexposed input image. This model expects an overexposed (0.9 $\geq$ bit density $\geq$ 0.75 )  image as input to recover the burst with high accuracy. 
    \item We assume that representative images of the burst are available for training as neural ODEs cannot extrapolate accurately. 
    \item We assume that the continuous label $\widetilde\theta$ of input image and target image are known beforehand.  
\end{itemize}

The drawbacks of our method are as follows -
\begin{itemize}
    \item Generative Adversarial Networks are known to be hard to optimize and converge. Since we adopt GAN framework, we inherit the optimization and convergence issues. For our experiments, we experimented with lower learning rates to stabilize the training process.
    \item In the main paper, we used Pix2Pix and CycleGAN as parent networks to derive our methods. These variations of GANs are not known for the best output image fidelity. Hence, we see several artefacts in the generated images. Using latest techniques and improvements in GAN literature we can achieve better fidelity especially for 512 x 512 experiments. 
    
\end{itemize}

\section*{A4 - Additional Qualitative Results on Synthetic Data}
In this section, we show additional qualitative results for exposure burst recovery and colorization. First, in Section S5.1 we show examples of exposure bursts recovered using our method for cases where input is \textbf{(a)} an over-exposed image \textbf{(b)} an under-exposed image.

\subsection*{A4.1 - Recovered Exposure Spectrum}

\begin{itemize}
    \item \textbf{Case 1 - With overexposed binary image input}
     - In Figure \ref{fig:overexp_burst} we show the results for burst recovery with an overexposed binary image as input.
        \begin{figure}
          \centering
           \includegraphics[width=0.9\textwidth,height=0.9\textheight,keepaspectratio]{sec/figs/over_exp_burst.jpg}
           \caption{Examples of recovered burst from overexposed input for AtomODE-CycleGAN and AtomODE-Pix2Pix.}
           \label{fig:overexp_burst}
        \end{figure}
    \item \textbf{Case 2 - With underexposed binary image input}
    - In Figure \ref{fig:underexp_burst} we show the results for burst recovery with an underexposed binary image as input and colorization results in Figure \ref{fig:underexp_colorized_image}.
        \begin{figure}
          \centering
        \includegraphics[width=0.9\textwidth,height=0.9\textheight,keepaspectratio]{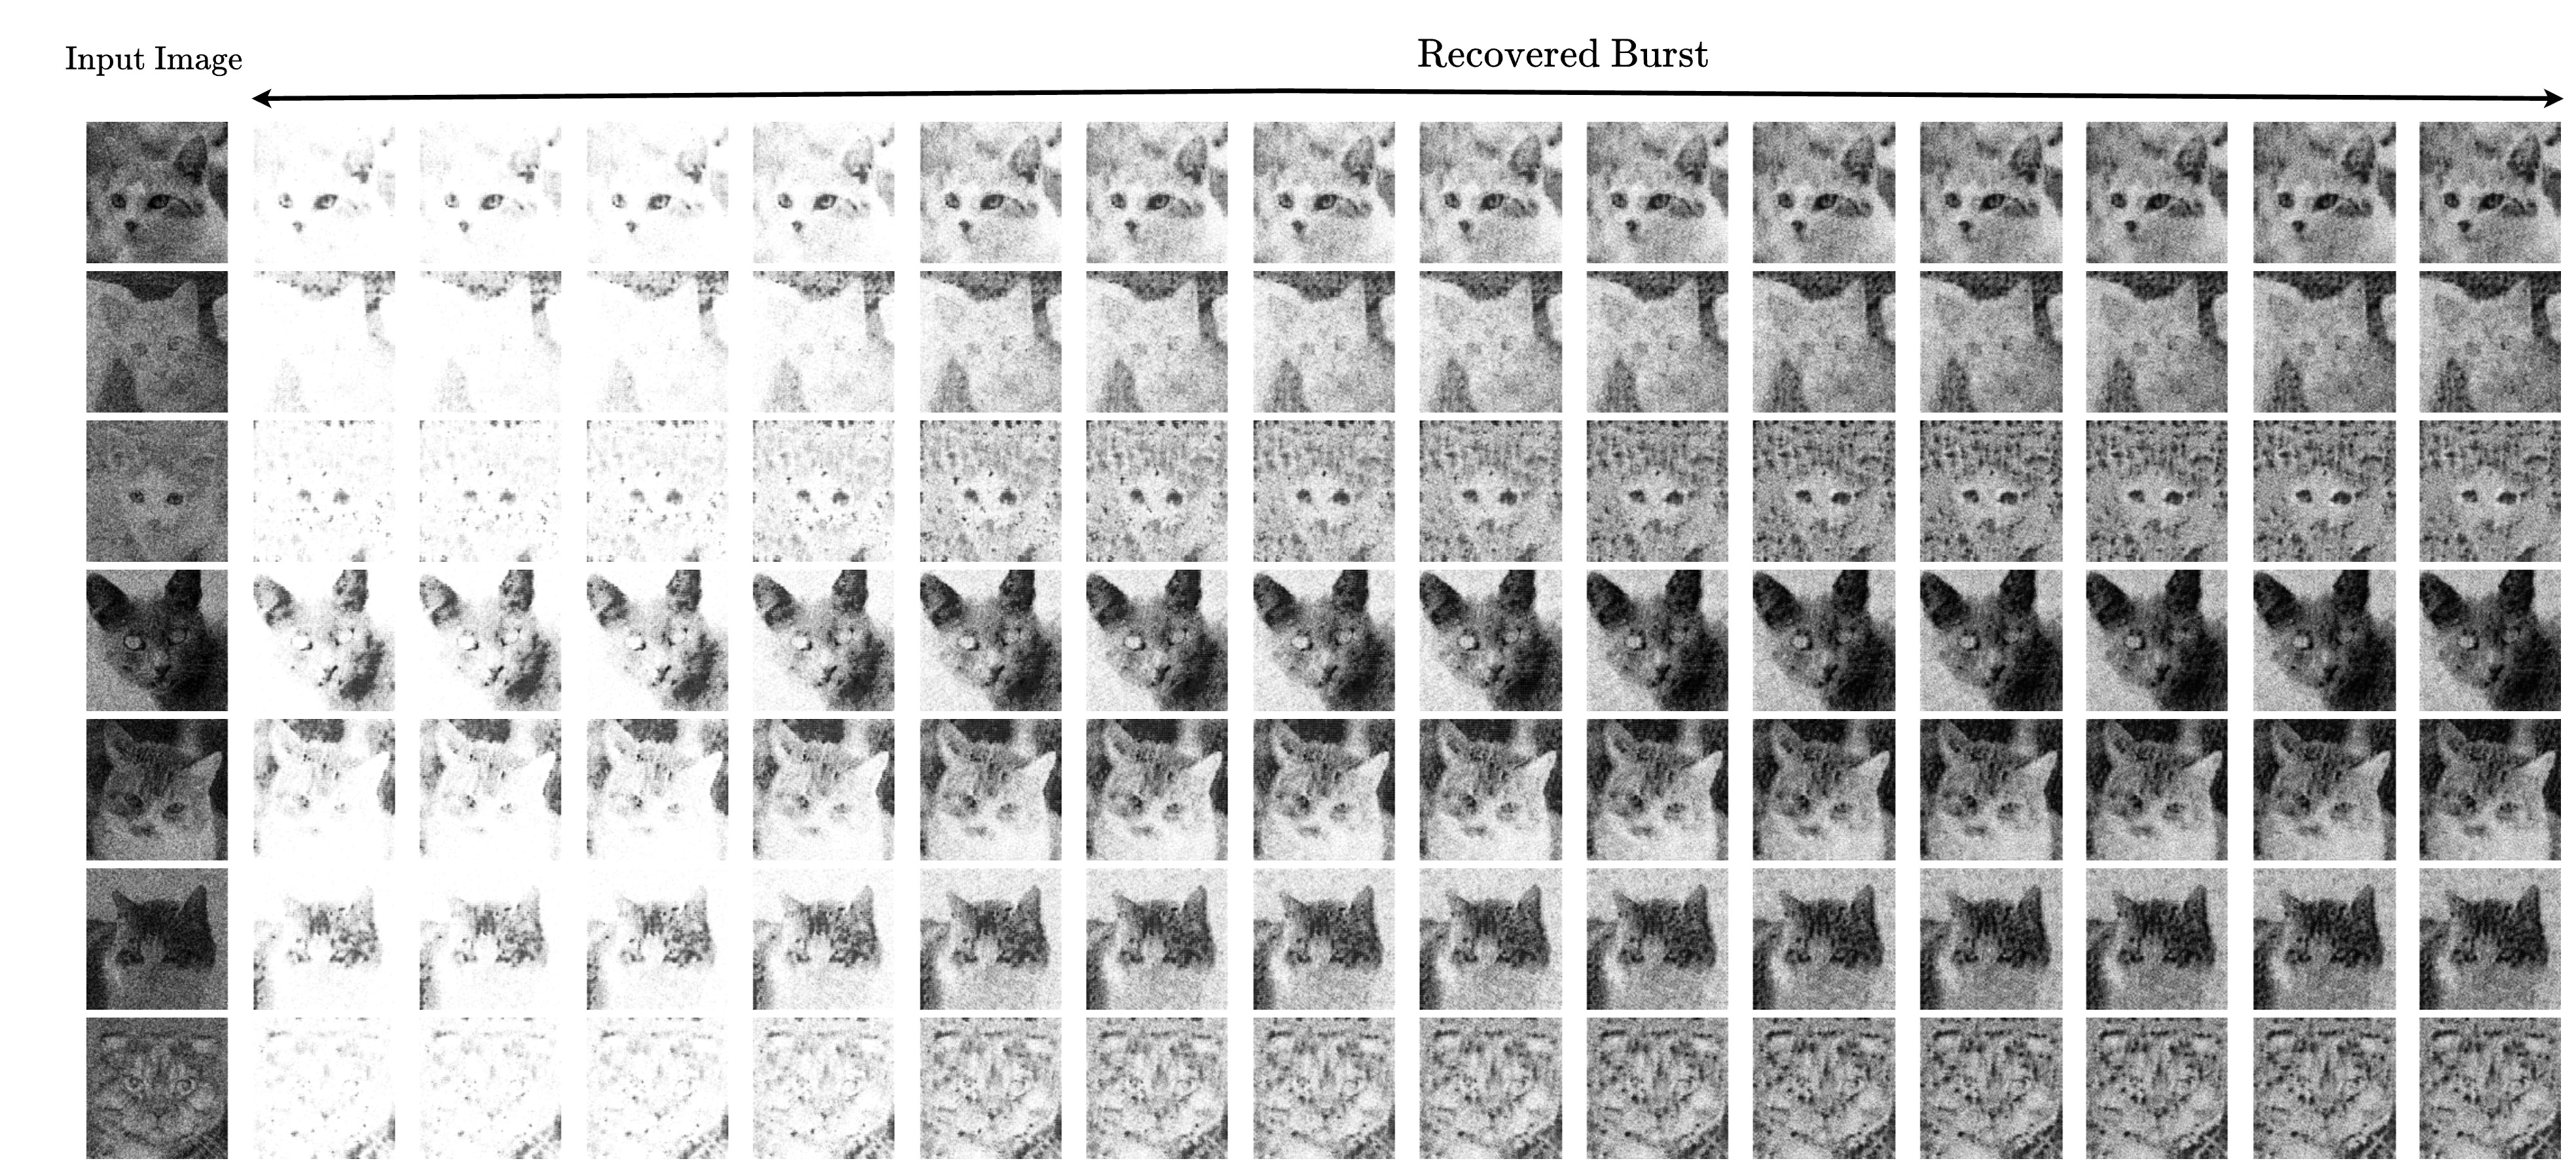}
           \caption{Examples of recovered burst from underexposed input for AtomODE-Pix2Pix.}
           \label{fig:underexp_burst}
        \end{figure}
        \begin{figure}
          \centering
        \includegraphics[width=0.9\textwidth,height=0.9\textheight,keepaspectratio]{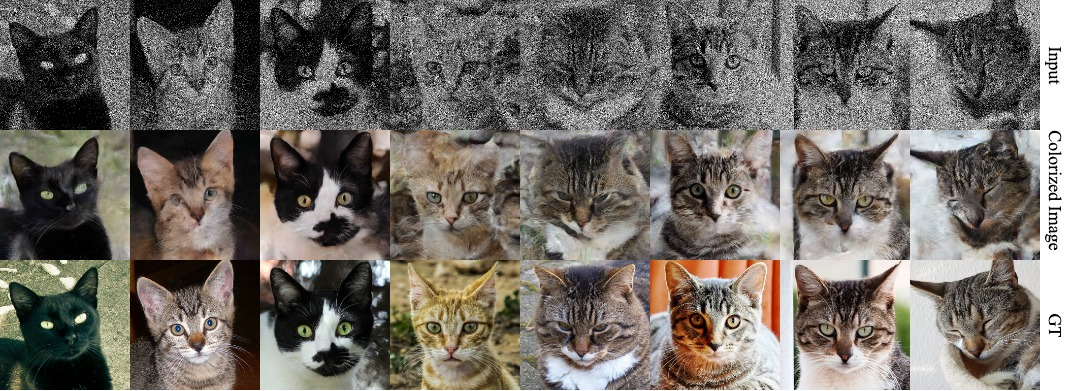}
           \caption{Examples of colorized image from underexposed input for using AtomODE-Pix2Pix as exposure correction method and Pix2PixHD as colorizer.}
           \label{fig:underexp_colorized_image}
        \end{figure}
\end{itemize}

\subsection*{A4.2 - Additional SIC Results and Colorization results for Overexposed Input}
    In Figure \ref{fig:sic_over}, we show some additional qualitative results for SIC for our methods, AtomODE-Pix2Pix, AtomODE-CycleGAN and competing methods. 
    \begin{figure}
          \centering
          \includegraphics[width=0.95\textwidth,height=\textheight,keepaspectratio]{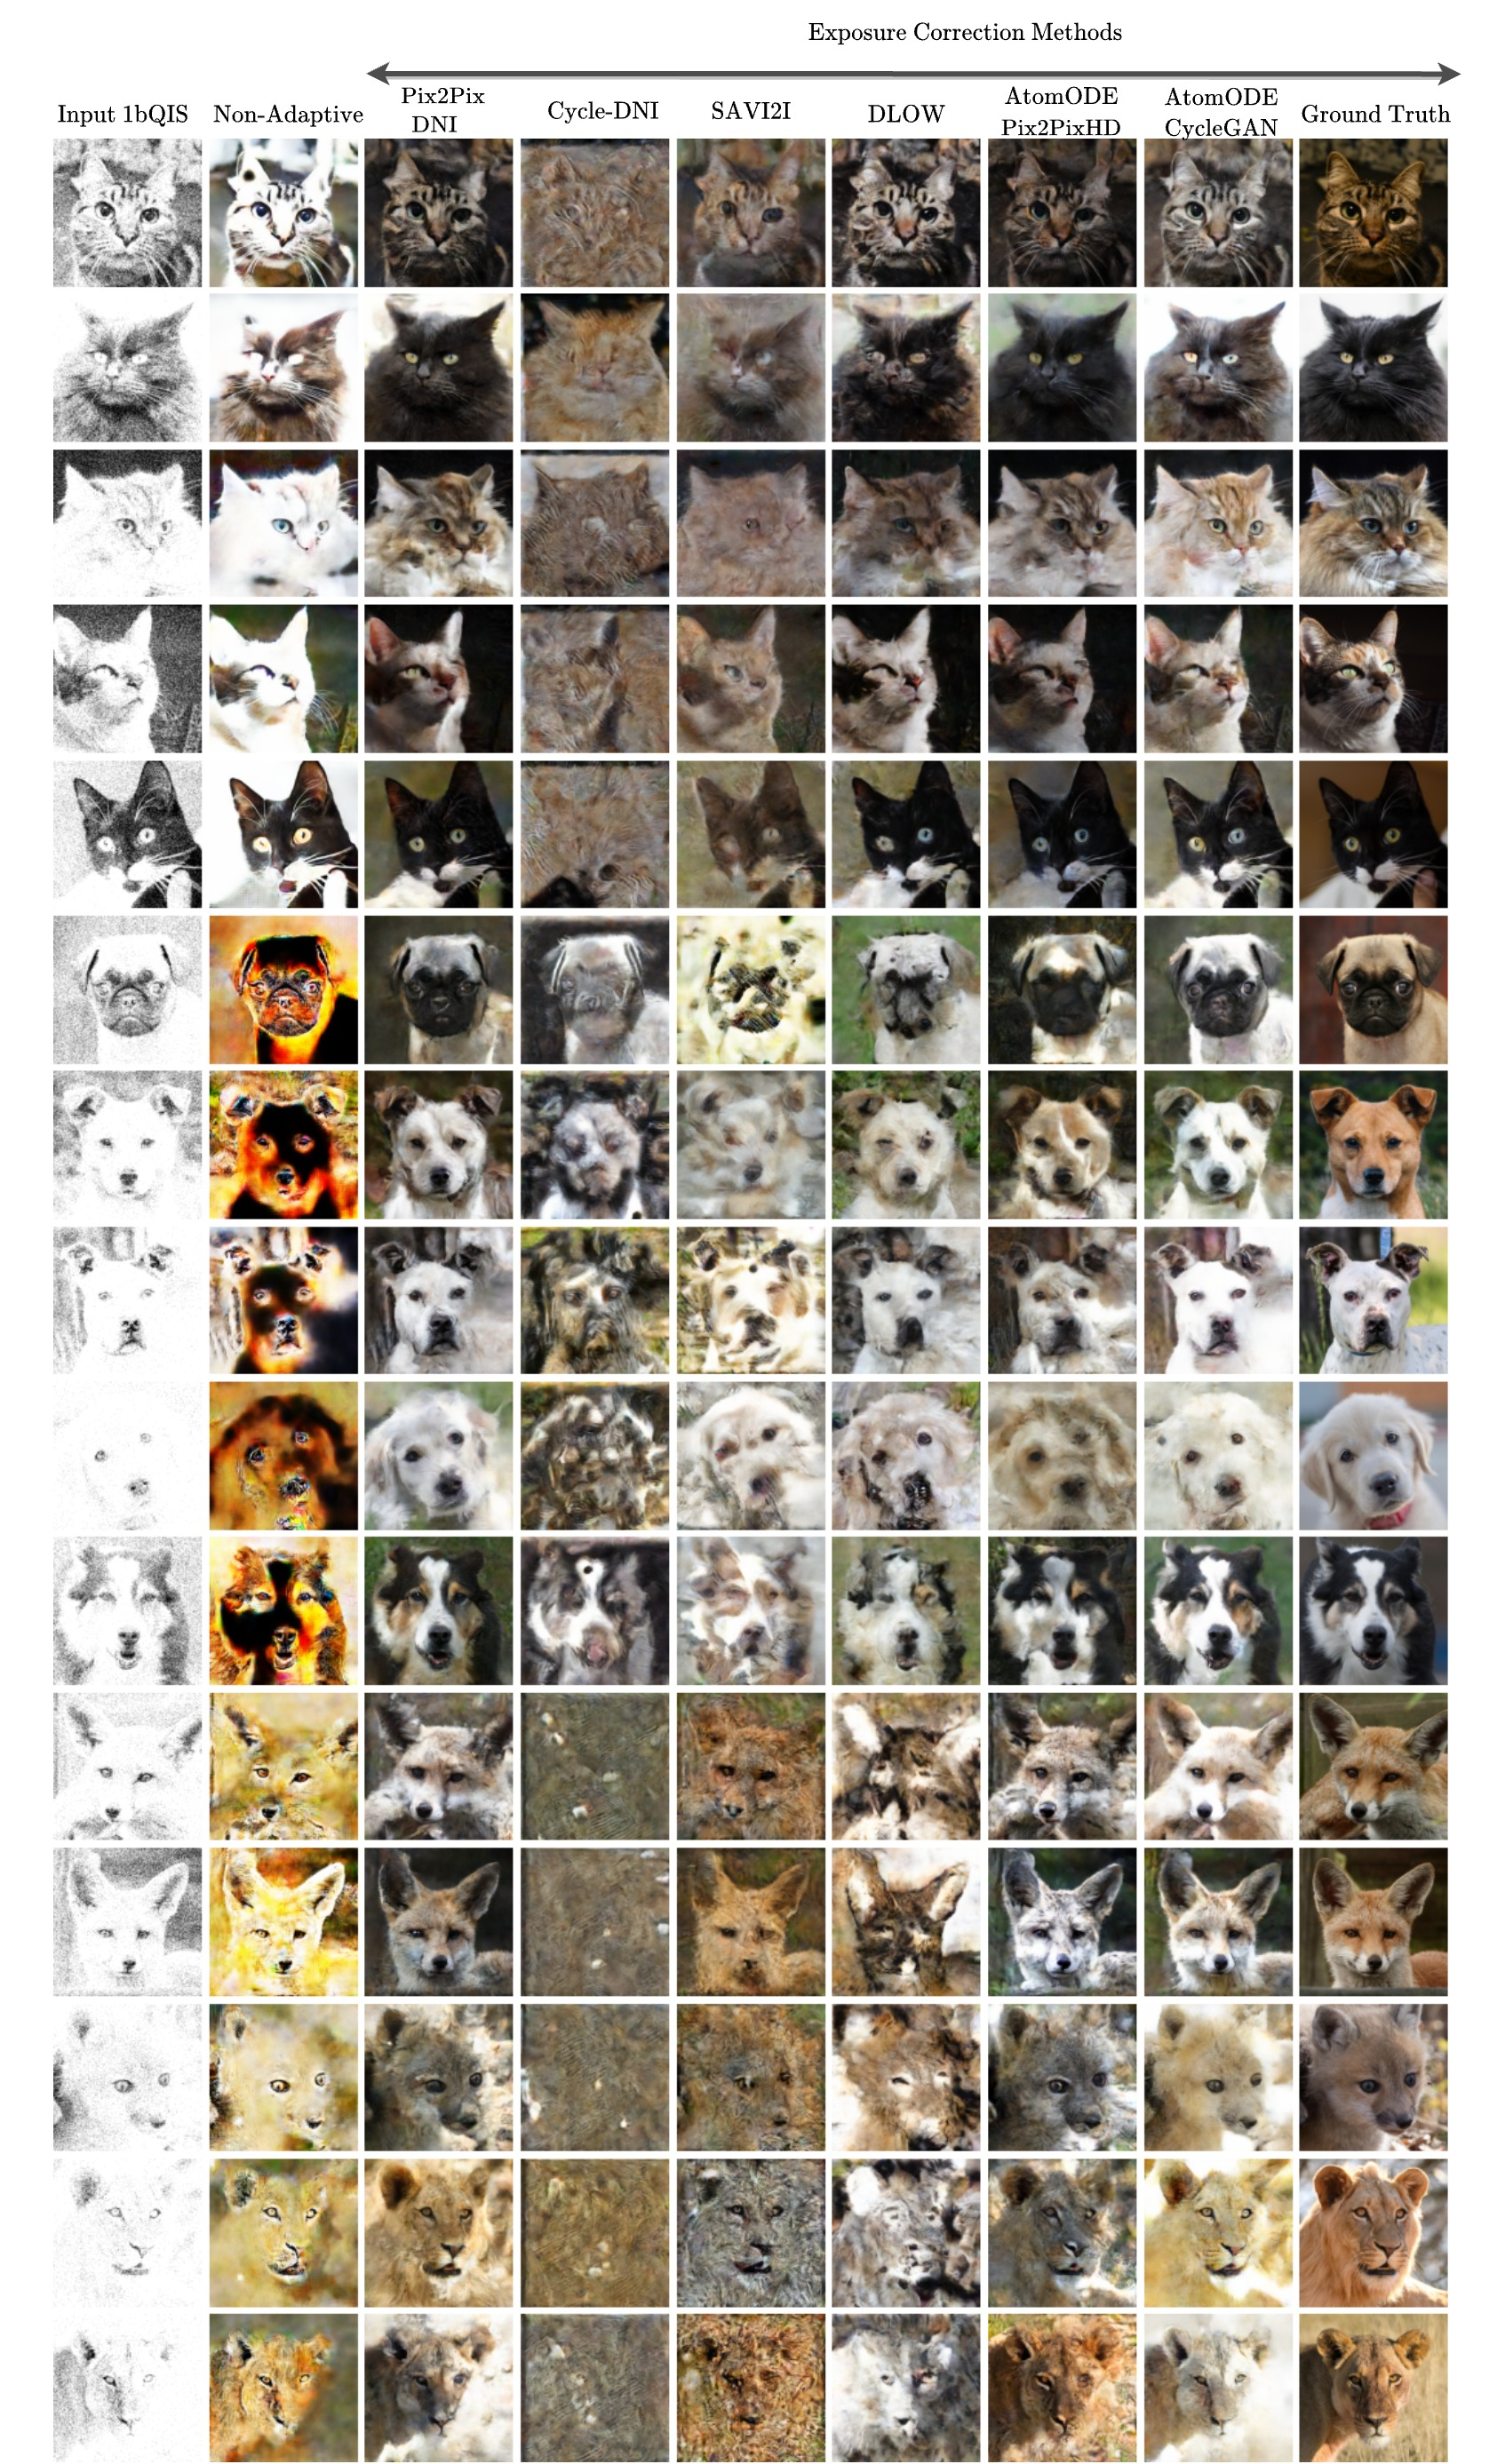}
           \caption{SIC results on AFHQ dataset using Pix2Pix colorizer.}
           \label{fig:sic_over}
    \end{figure}
\section*{A5 - Experiment Setup for Real World Image Capture}

This section describes the experimental setup we build to capture the real-world images used in this paper. As in Figure~\ref{fig:fig3}, our setup consists of a monochrome camera that is either a CMOS (Basler ace acA2440-35um) or a QIS (Gigajot PathFinder prototype camera~\cite{ma2017photon}), an RGB camera (Basler ace acA2440-35uc), and a flat target that contains a pattern from the AFHQ dataset and a series of April Tags. We take images of the target using both cameras and warp the RGB image to align with the monochrome image by calculating the homography from the detected April Tags. When mounting the setup, we ensure that the monochrome camera is approximately front parallel to the target, so that the pattern is rectangular in the monochrome image and can be naively cropped out. This is because we want to avoid warping the monochrome image; the interpolation required by warping can alter the statistical property of the pixel values of the warped image. 
\begin{figure}
          \centering
           \includegraphics[width=0.6\textwidth,height=0.6\textheight,keepaspectratio]{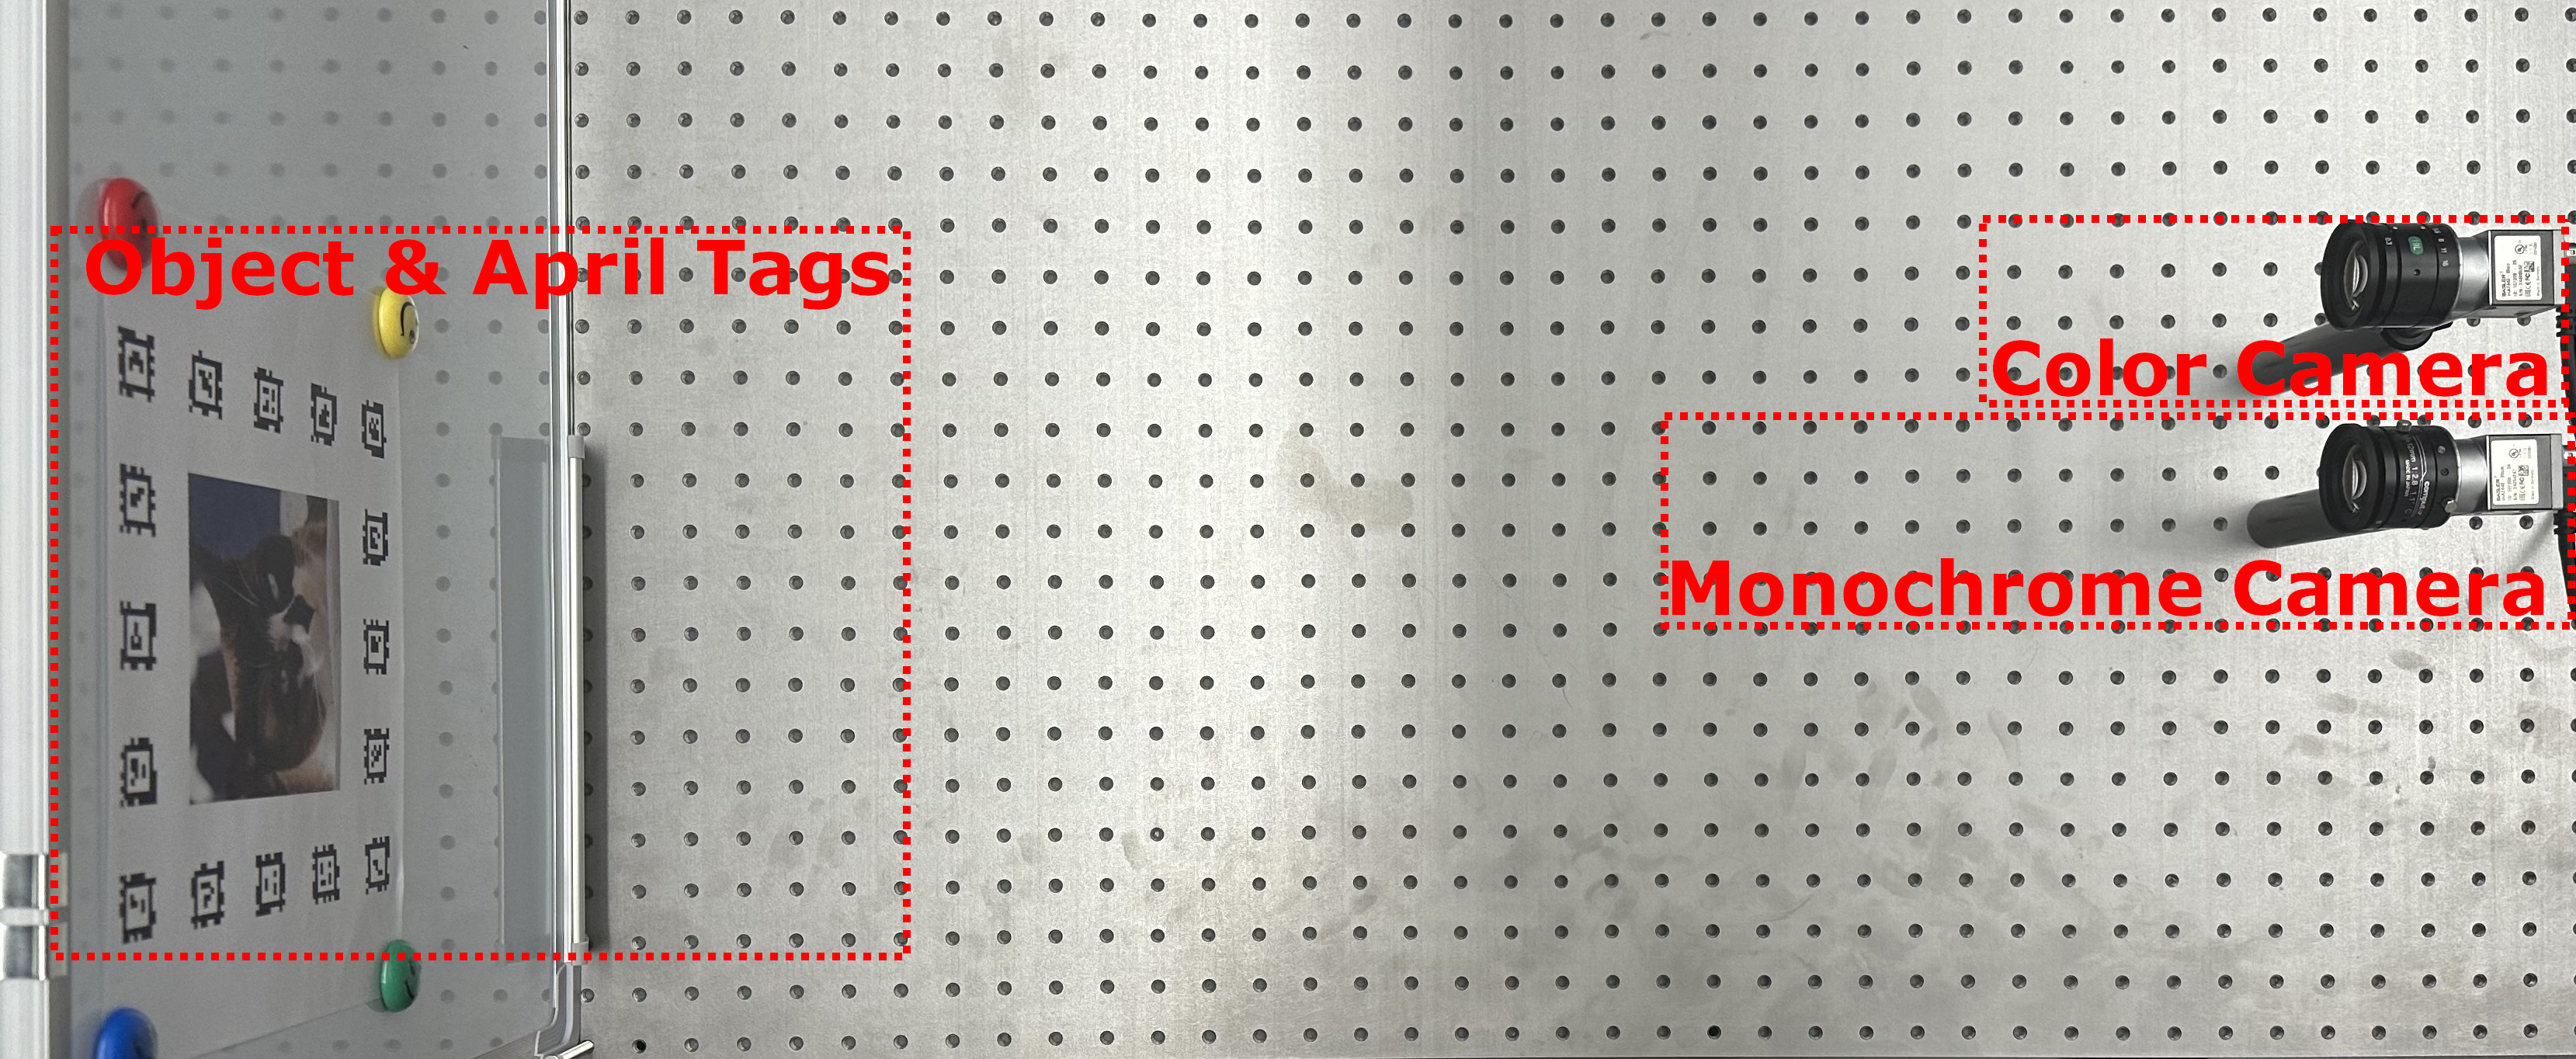}
           \caption{The experimental setup.}
           \label{fig:fig3}
\end{figure}

\begin{figure}%
    \centering
    \subfloat[\centering RGB Image]{{\includegraphics[width=5cm]{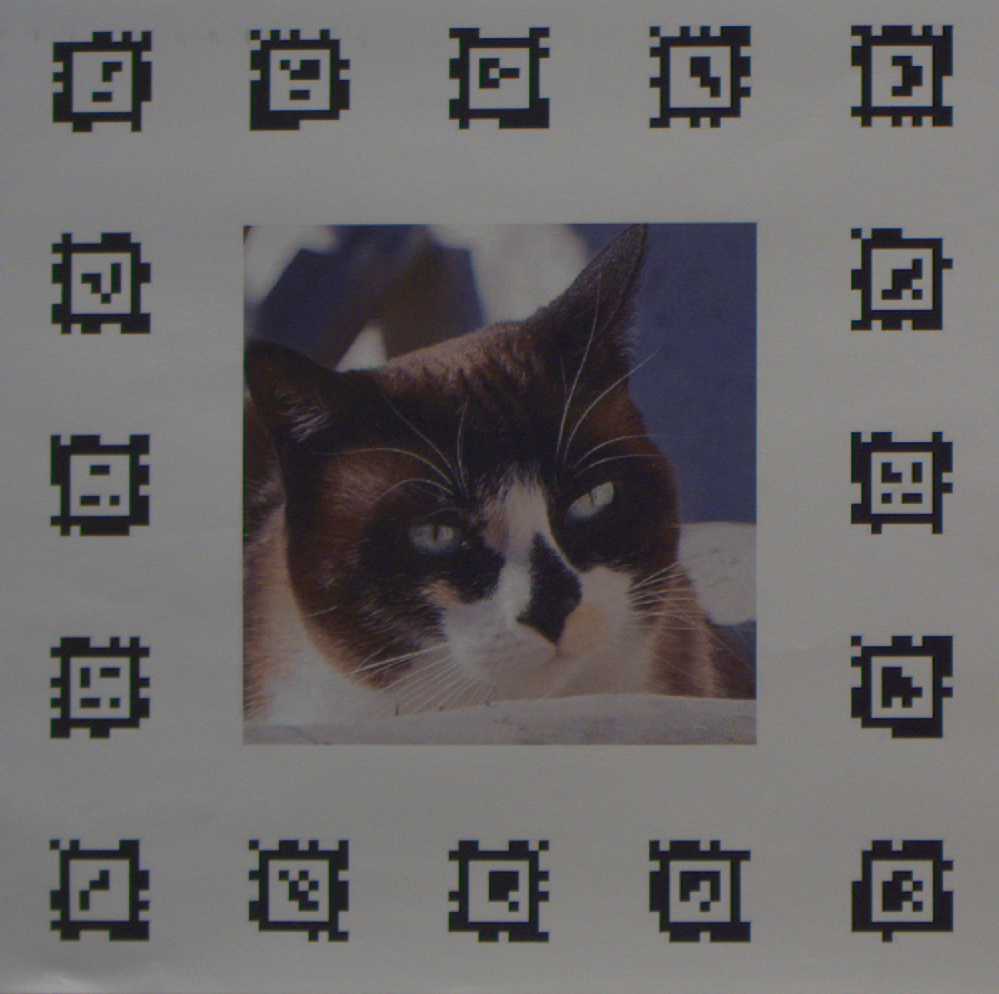} }}%
    \qquad
    \subfloat[\centering Monochrome Image]{{\includegraphics[width=5cm]{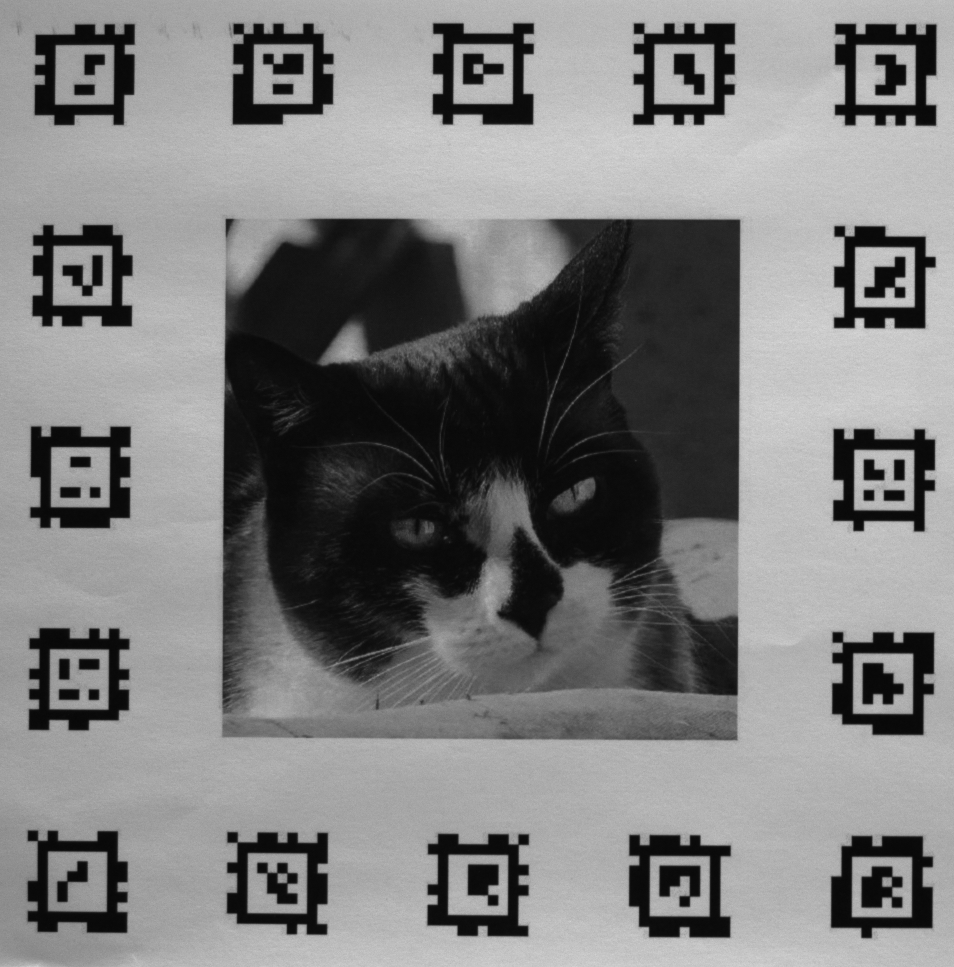} }}%
    \caption{Sample images taken by the RGB camera and the monochrome camera without alignment.}%
    \label{fig:example}%
\end{figure}

We use the following parameters in our image capture process. The CMOS monochrome camera was set with an exposure time of 464 us, a gain of 24 dB, a digital shift of 0, and a pixel format of Mono 12. We noticed that when the gain is 24 dB, each gray level of the pixel value corresponds to one excited electron on the photodiode. 
The RGB camera was set with an exposure time of 30000 us, a gain of 0 dB, a digital shift of 0, and a pixel format of Bayer RG 12. Lastly, the QIS camera was set with an exposure time of 74 us, a gain of 0 dB, a digital shift of 0, and a pixel format of Mono 14.

To fine-tune and test our model on real data, we capture a total of 125 image pairs, among which 100 are for fine-tuning and 25 are for testing. For each fine-tuning and testing pair, we use different targets with patterns sampled from the training and testing set of AFHQ dataset, respectively. Each image pair $i$ for fine-tuning consists of a CMOS monochrome image $I^{\text{Mono}}_{i}$ and an RGB image $I^{\text{RGB}}_{i}$ of the same target captured using the previously stated camera settings, $i = 1,\cdots, 100$. Similarly, for the testing data, we collect 25 pairs of CMOS monochrome images $I^{\text{Mono}}_{i}$ and RGB images $I^{\text{RGB}}_{i}, i = 101, \cdots, 125$, as well as 25 pairs of QIS images $I^{\text{QIS}}_{i}$ and RGB images $I^{\text{RGB}}_{i}, i=126,\cdots, 150$. 

After the data capture, we need to translate the pixel value of each image to represent the number of photons received by each pixel. For the monochrome CMOS images $ I^{\text{Mono}}_{i}$, we can relate the gray level of each pixel $I$ to the number of photons using the following formula:

\begin{equation}
    X = G\times I / QE.
    \label{eq:cmos}
\end{equation}

Here, $X$ is the number of photons recorded by a pixel in an exposure period plus the dark noise, $G$ is the value of the gain ratio, $I$ is the value of the pixel, and $QE$ represents quantum efficiency. Based on our previous discussion, in our setup, the value of $G$ is 1 in our experiment. The quantum efficiency $QE$ is $0.68$ according to the datasheet. By applying Equation~\ref{eq:cmos}, we can convert the pixel value of each CMOS image $I^{\text{Mono}}_{i}$ to the number of photons received in each pixel $X$.

As for the QIS camera, we first calibrate the dark current $I_{\text{dark}}$ and the photo response non-uniformity (PRNU) function $\text{CRF()}$ on the raw data. Subsequently, we convert the calibrated data to photon counts by taking into account the quantum efficiency (QE) based on the following equation:
\begin{equation}
    I = \text{ADC}\{ \text{Clip}\{G \times \text{Possion}(ET \times QE \times (\text{CRF}(X) + I_{\text{dark}})) \} \} + \text{Gaussian}(0, \sigma^2_{\text{real\_noise}}),
\end{equation}
where $X$ is the number of photons received by a pixel in an exposure period, $G$ is the gain ratio, $I$ is the pixel value of the QIS camera,  $QE$ is quantum efficiency, ET is the exposure time, and ADC represents the analog to digital converter. We can directly obtain the number of photons $X$ received by each pixel directly using the translation equation provided by the manufacturer~\cite{ma2017photon}.

\section*{A6 - Details about finetuning on real-world data}
The results reported for real world CMOS images we use a finetuned colorizer. We first recover the exposure burst using AtomODE-CycleGAN and use the image at index $\tau = 10$ as input 1bQIS image and corresponding CMOS RGB image as target image for finetuning. We finetune the colorizer for 50 epochs on 100 training image pairs (1bQIS and corresponding CMOS RGB image).
